# Supplementary material for: MeMOT: Multi-Object Tracking with Memory
Source: arXiv:2203.16761 source file (2022-03-31)
Supplement: Supplementary file 1 [file appendix_detail_mot.tex]

\begin{table*}[t!]
    \small
    \centering
    \setlength\tabcolsep{4.5pt}
    \begin{tabular}{c|cccccccccccc}
    \toprule[1.5pt]
        \textbf{Sequence} &\textbf{MOTA}  $\uparrow$ & \textbf{IDF1} $\uparrow$ & \textbf{HOTA} $\uparrow$ & \textbf{MT} $\uparrow$ & \textbf{ML} $\downarrow$ & \textbf{FP} $\downarrow$ & \textbf{FN} $\downarrow$ & \textbf{Recall} $\uparrow$ & \textbf{Precision} $\uparrow$ & \textbf{AssA} $\uparrow$ & \textbf{DetA} $\uparrow$ & \textbf{IDsw} $\downarrow$  \\\hline
         \multicolumn{13}{c}{\textbf{MOT16} \cite{milan2016mot16}} \\\hline\hline
         MOT16-01 & 56.7 & 55.9 & 46.3 & 8 & 7 & 214 & 2527 & 60.5 & 94.8 & 45.7 & 47.0 & 28\\
         MOT16-03 & 85.3 & 79.7 & 64.9 & 134 & 0 & 8257 & 6971 & 93.3 & 92.2 & 62.1 & 68.2 & 123\\
         MOT16-06 & 60.2 & 62.7 & 50.7 & 84 & 51 & 872 & 3583 & 68.9 & 90.2 & 51.1 & 55.5 & 141\\
         MOT16-07 & 64.9 & 52.9 & 45.9 & 23 & 4 & 1008 & 4623 & 71.7 & 92.1 & 41.5 & 78.1 & 105\\
         MOT16-08 & 48.1 & 44.4 & 41.0 & 21 & 4 & 2407 & 6059 & 63.8 & 81.6 & 36.8 & 46.7 & 226\\
         MOT16-12 & 63.4 & 66.9 & 55.4 & 36 & 18 & 510 & 2476 & 70.2 & 91.9 & 57.2 & 53.9 & 50 \\
         MOT16-14 & 46.7 & 51.7 & 38.5 & 35 & 42 & 1327 & 8356 & 54.8 & 88.4 & 38.9 & 38.6 & 172\\
         Overall & 72.6 & 69.7 & 57.4 & 341 & 126 & 14595 & 34595 & 81.0 & 91.0 & 55.7 & 59.5 & 845 \\\hline
         \multicolumn{13}{c}{\textbf{MOT17} \cite{milan2016mot16}} \\\hline\hline
         MOT17-01 & 56.5 & 55.8 & 46.2 & 8 & 8 & 205 & 2570 & 60.2 & 95.0 & 45.9 & 46.7 & 28 \\
         MOT17-03 & 85.8 & 79.8 & 65.1 & 134 & 0 & 7973 & 6790 & 93.5 & 92.5 & 62.2 & 68.5 & 123 \\
         MOT17-06 & 61.4 & 62.4 & 50.8 & 83 & 50 & 723 & 3680 & 68.8 & 91.8 & 50.2 & 51.6 & 146\\
         MOT17-07 & 63.1 & 51.5 & 44.8 & 22 & 8 & 964 & 5151 & 69.5 & 92.4 & 38.3 & 52.7 & 111 \\
         MOT17-08 & 52.0 & 42.1 & 37.4 & 25 & 12 & 783 & 9088 & 57.0 & 93.9 & 32.8 & 43.3 & 275 \\
         MOT17-12 & 62.2 & 66.0 & 54.6 & 37 & 21 & 442 & 2781 & 67.9 & 93.0 & 56.9 & 52.7 & 53\\
         MOT17-14 & 46.7 & 51.7 & 38.5 & 35 & 42 & 1317 & 8356 & 54.8 & 88.5 & 38.9 & 38.6 & 172 \\
         Overall & 72.5 & 69.0 & 56.9  & 1032 & 423 & 37221 & 115248 & 79.6 & 92.3 & 55.2 & 58.9 & 2724  \\\hline
         \multicolumn{13}{c}{\textbf{MOT20} \cite{dendorfer2020mot20}} \\\hline\hline
        MOT20-04& 84.8 & 80.1 & 65.5 & 540 & 19& 14628 & 137983 & 90.3 & 94.4 & 62.4 & 69.0 & 468\\
        MOT20-06 & 39.9 & 46.4 & 35.9 & 68 & 78 & 17579 & 26577 & 53.8 & 80.2 & 35.3 & 36.8 & 918\\
        MOT20-07 & 74.2 & 70.5 & 58.7 & 80 & 4 & 3365 & 61336 & 84.7 & 89.3 & 56.0 & 62.0 & 138\\
        MOT20-08 & 25.5 & 38.3 & 30.9 & 26 & 76 & 12310 & 5049 & 41.9 & 72.5& 34.5 & 28.0 & 414\\
        Overall & 63.7 & 66.1 & 54.1 & 714 & 177 & 47882 & 45021 & 73.3 & 88.8 & 55.0& 53.5 & 1938\\\hline
    \bottomrule[1.5pt]
    \end{tabular}
 \vspace{-2.0mm}
    \caption{Performance of each sequence in MOT Challenge benchmarks.}
    \label{tab:MOTexp_seq}
    \vspace{-1.5mm}
\end{table*}
